# Supplementary material for: AssemblyComplete: 3D Combinatorial Construction with Deep Reinforcement Learning
Source: arXiv:2410.15469 source file (2024-10-20)
Supplement: Supplementary file 1 [file appendix.tex]

\section{Experimental Details}
\label{sec: experiment details}

In this appendix, we provide the details of the experiments in Section~\ref{sec: experiment details}.
